# Supplementary material for: Density Functional Leveraged Tight-binding Insights into Inorganic Halide Perovskites
Source: arXiv:2501.06503 source file (2025-01-11)
Supplement: Supplementary file 1 [file St1.tex]

% \begin{table}[H]
% \caption{\label{Shannonradii}Some parameters that influence the structural and transport properties of perovskites}
% \begin{ruledtabular}
% \begin{tabular}{lrr}
 
%  Element & Shannon Radius (\AA) & Electronegativity (Mulliken's scale) \\
%          \hline
%          Cs     & 1.88 &  2.19 \\
         
%          Pb     &  1.19   & 3.89 \\
         
%          Br     &  1.96   &  7.56 \\
         
%          I      & 2.20 & 6.76 \\
% \end{tabular}
% \end{ruledtabular}
% \end{table}
